# Supplementary material for: Measuring nuclear spin qubits by qudit-enhanced spectroscopy in Silicon Carbide
Source: arXiv:2310.15557 source file (2023-10-24)
Supplement: Supplementary file 1 [file Supplementary.pdf]

# Supplemental Material for "Measuring nuclear spin qubits by qudit-enhanced spectroscopy in Silicon Carbide"

Erik Hesselmeier,[1] Pierre Kuna,[1] István Takács,[2,3] Viktor Ivády,[2,3,4] Wolfgang Knolle,[5] Nguyen Tien Son,[4] Misagh Ghezellou,[4] Jawad Ul-Hassan,[4] Durga Dasari,[1] Florian Kaiser,[6,7] Vadim Vorobyov,[1,*] and Jörg Wrachtrup[1,8]

[1] *3rd Institute of Physics, IQST, and Research Centre SCoPE, University of Stuttgart, Stuttgart, Germany*
[2] *Eötvös Loránd University, Egyetem tér 1-3, H-1053 Budapest, Hungary*
[3] *MTA–ELTE Lendület "Momentum" NewQubit Research Group, Pázmány Péter, Sétány 1/A, 1117 Budapest, Hungary*
[4] *Department of Physics, Chemistry and Biology, Linköping University, Linköping, Sweden*
[5] *Department of Sensoric Surfaces and Functional Interfaces, Leibniz-Institute of Surface Engineering (IOM), Leipzig, Germany*
[6] *Materials Research and Technology (MRT) Department, Luxembourg Institute of Science and Technology (LIST), 4422 Belvaux, Luxembourg*
[7] *University of Luxembourg, 41 rue du Brill, L-4422 Belvaux, Luxembourg*
[8] *Max Planck Institute for solid state physics, Stuttgart, Germany*

## I. DETERMINATION OF THE HYPERFINE COUPLING COEFFICIENTS

The V2-Hamiltonian is described by the following equation (neglecting the nuclear-nuclear interactions):

$$H = D(S_z^2 - \frac{1}{3}(S(S+1))) + \vec{B}(g_e\hat{S} + g_n\hat{I}) + \hat{S}A\hat{I} \tag{1}$$

where $D$ is the zero field splitting, $S = 3/2$ the spin number, $g_e$ and $g_n$ the electron and nuclear gyromagnetic factors respectively. $\hat{S}$ is the spin operator of the electron spin, $\hat{I}$ the spin operator of the nuclear spin and $\mathbf{A}$ the 3x3 hyperfine tensor. Thus, $D(S_z^2 - \frac{1}{3}(S(S+1)))$ is the zero-field splitting, $\vec{B}\cdot(g_e\hat{S} + g_n\hat{I})$ the Zeeman shift of the electron and nuclear spin, and $\hat{S}\mathbf{A}\hat{I}$ the coupling between the nuclear and the electron spin. The value of $g_e$ is well known to be 2.804 MHz/Tesla and the gyromagnetic factor of the nuclei are $g_n(^{29}\mathrm{Si}) = -8.465e\text{-}4\,\mathrm{MHz/Tesla}$ and $g_n(^{13}\mathrm{C}) = 10.705e\text{-}4\,\mathrm{MHz/Tesla}$.

To extract the hyperfine terms, we first measure all the electron and nuclear transition frequencies (see main text). We proceed by fitting the Hamiltonian (eq. 1) using the python module "lmfit". The free parameters in the Hamiltonian are $D, B, \theta, \phi, A_{xx}, A_{yy}, A_{zz}, A_{xy}, A_{xz}, A_{yz}$ where $B$ is the intensity of the magnetic field, $\theta$ the polar angle and $\phi$ the azimutal angle. Each time a new set of free parameters is tested, we calculate the new Hamiltonian and its eigenenergies. From there we can calculate the transition energies and compare them to the measured transition frequencies. These are then compared to the measured transition frequencies with the cost function being the squared sum of the difference between the calculated and measured frequencies. We used the default minimization algorithm of "lmfit" which is "Nelder Mead minimization".

To characterize the stability of the fit, we added some random noise to the measured transitions and to the initial guess of the fit. The highest amplitude of the transition noise is 50 kHz and the highest noise on the initial fit parameters is 20% of their original value. We repeat this procedure 1000 times to get significant statistics on the fit parameter stability. We find that the parameters $D, B, \theta and A_{zz}$ have a standard deviation of less than 5 %. $A_{xx}$ and $A_{yy}$ show a standard deviation of 20 %. The other parameters $A_{yx}, A_{xz}, A_{yz}$ and $\phi$ are very unstable: their standard deviation is much higher than 50%.

* v.vorobyov@pi3.uni-stuttgart.de

## II. TOMOGRAPHY OF THE STATE POPULATIONS

### 1. *Method for spin $S = \frac{3}{2}$*

To infer the polarization of the electronic states, we used the method described in the previous paper by Nagy et al. [1]: The visibility of all electron transitions ($\mathrm{MW}_L$, $\mathrm{MW}_C$, $\mathrm{MW}_R$) were measured. The $\mathrm{MW}_C$ transition doesn't change the readout, hence an additional $\mathrm{MW}_R$ $\pi$ pulse was applied, to map the electron population to the $m_s = 3/2$ state. The visibility $V = (I_{max} - I_{min})/(I_{max} + I_{min})$ of the oscillations is calculated for these scenarios, and with overall probability equalling 1, the system of equations is set.

$$\begin{aligned}
V_L &= \frac{p(-\frac{3}{2}) - p(-\frac{1}{2})}{2p(\frac{3}{2}) + p(-\frac{3}{2}) + p(-\frac{1}{2})} \\
V_C &= \frac{p(\frac{1}{2}) - p(-\frac{1}{2})}{2p(-\frac{3}{2}) + p(\frac{1}{2}) + p(-\frac{1}{2})} \\
V_R &= \frac{p(\frac{3}{2}) - p(\frac{1}{2})}{2p(-\frac{3}{2}) + p(\frac{3}{2}) + p(\frac{1}{2})} \\
p(-\frac{3}{2}) &+ p(-\frac{1}{2}) + p(\frac{3}{2}) + p(\frac{1}{2}) = 1.
\end{aligned} \tag{2}$$

### 2. *Adding the hyperfine nuclear spin sub-manifold populations*

When adding a nuclear spin to the picture, we get additional parameters, which define sub-manifold relative populations. It is useful to write them in the form:

$$p(m_s, \uparrow) + p(m_s, \downarrow) = p(m_s),\ m_s = \pm\frac{3}{2}, \pm\frac{1}{2} \tag{3}$$

Finally, the additional 6 equations could be obtained from selective Rabi oscillations:

$$\begin{aligned}
V_{L1} &= \frac{p(-\frac{3}{2},\downarrow) - p(-\frac{1}{2},\downarrow)}{2p(\frac{3}{2}) + 2p(-\frac{3}{2},\uparrow) + p(-\frac{1}{2},\downarrow) + p(-\frac{3}{2},\downarrow)} \\
V_{L2} &= \frac{p(-\frac{3}{2},\uparrow) - p(-\frac{1}{2},\uparrow)}{2p(\frac{3}{2}) + 2p(-\frac{3}{2},\downarrow) + p(-\frac{1}{2},\uparrow) + p(-\frac{3}{2},\uparrow)} \\
V_{R1} &= \frac{p(\frac{3}{2},\downarrow) - p(\frac{1}{2},\downarrow)}{2p(-\frac{3}{2}) + 2p(\frac{3}{2},\uparrow) + p(\frac{1}{2},\downarrow) + p(\frac{3}{2},\downarrow)} \\
V_{R2} &= \frac{p(\frac{3}{2},\uparrow) - p(\frac{1}{2},\uparrow)}{2p(-\frac{3}{2}) + 2p(\frac{3}{2},\downarrow) + p(\frac{1}{2},\uparrow) + p(\frac{3}{2},\uparrow)} \\
V_{C1} &= \frac{p(\frac{1}{2},\uparrow) - p(-\frac{1}{2},\uparrow)}{2p(-\frac{3}{2}) + 2p(\frac{1}{2},\downarrow) + p(\frac{1}{2},\uparrow) + p(-\frac{1}{2},\uparrow)} \\
V_{C2} &= \frac{p(\frac{1}{2},\downarrow) - p(-\frac{1}{2},\downarrow)}{2p(-\frac{3}{2}) + 2p(\frac{1}{2},\uparrow) + p(\frac{1}{2},\downarrow) + p(-\frac{1}{2},\downarrow)}
\end{aligned} \tag{4}$$

All in all we have now 14 equations, for 12 unknowns, some of the equations are redundant. The solution of this system could be obtained numerically, with certain condition on the variables, e.g. $p \in [0, 1]$. Also, the system could

be solved, by first finding $p(m_s)$ by solving first four equations,

$$p\left(-\frac{1}{2}\right) = \frac{V_C V_L V_R + 3V_C V_L - V_C V_R + V_C + 3V_L V_R + V_L + V_R - 1}{4(V_C V_L V_R - V_C + V_L V_R - 1)}$$
$$p\left(-\frac{3}{2}\right) = \frac{-3V_C V_L V_R - V_C V_L - V_C V_R + V_C - V_L V_R - 3V_L + V_R - 1}{4(V_C V_L V_R - V_C + V_L V_R - 1)}$$
$$p\left(\frac{1}{2}\right) = \frac{5V_C V_L V_R - V_C V_L + 3V_C V_R - 3V_C + 3V_L V_R + V_L + V_R - 1}{4(V_C V_L V_R - V_C + V_L V_R - 1)}$$
$$p\left(\frac{3}{2}\right) = \frac{V_C V_L V_R - V_C V_L - V_C V_R - 3V_C - V_L V_R + V_L - 3V_R - 1}{4(V_C V_L V_R - V_C + V_L V_R - 1)}$$

and then splitting the 8 equations in two groups for $+\frac{3}{2}, +\frac{1}{2}$ and $-\frac{3}{2}, -\frac{1}{2}$ electron sub-manifolds, which reduces the complexity substantially. Unfortunately, the set of equations is degenerate, which could be seen by solving the $p(-\frac{3}{2}, \uparrow) = p(-\frac{3}{2}) - p(-\frac{3}{2}, \downarrow)$ and substituting into the $V_{L1}$ and $V_{L2}$:

$$V_{L1} = \frac{-p(-\frac{1}{2}) + p(-\frac{3}{2}) + p(-\frac{1}{2}, \uparrow) - p(-\frac{3}{2}, \uparrow)}{p(-\frac{1}{2}) + p(-\frac{3}{2}) + 2p(\frac{3}{2}) - p(-\frac{1}{2}, \uparrow) + p(-\frac{3}{2}, \uparrow)} \tag{5}$$
$$V_{L2} = \frac{-p(-\frac{1}{2}, \uparrow) + p(-\frac{3}{2}, \uparrow)}{2p(-\frac{3}{2}) + 2p(\frac{3}{2}) + p(-\frac{1}{2}, \uparrow) - p(-\frac{3}{2}, \uparrow)} \tag{6}$$

From here we can solve for $p(-\frac{1}{2}, \uparrow) - p(-\frac{3}{2}, \uparrow)$ from both equations, substract from each other, and cancel one of the equations. Similarly, one of the equations $R1, R2$ and $C1, C2$ could be reduced to only one this way. The resulting 3 equations, is not enough to solve for 4 probabilities of nuclear spin $\uparrow$. We can add to the system a visibility in nuclear Rabi oscillations at $m_s = -\frac{1}{2}(+\frac{1}{2})$ with a CNOT at L1(R1) transition (a nuclear selective *pi* pulse), with some approximations regarding the achievable contrast, due to state hybridisations.

$$V_n^{m_s=-\frac{1}{2}} = \frac{p(-\frac{1}{2}, \downarrow) - p(-\frac{1}{2}, \uparrow)}{p_{3/2} + p(-\frac{3}{2}, \uparrow) + \frac{1}{2}p_{-1/2}} \tag{7}$$
$$V_n^{m_s=+\frac{1}{2}} = \frac{p(\frac{1}{2}, \downarrow) - p(\frac{1}{2}, \uparrow)}{p_{-3/2} + p(\frac{3}{2}, \uparrow) + \frac{1}{2}p_{1/2}} \tag{8}$$
$$\tag{9}$$

In summary, now we can close the system of equations for $-\frac{1}{2}, -\frac{3}{2}$ subdomain:

$$V_n^{ms=-\frac{1}{2}} = \frac{p(-\frac{1}{2}, \downarrow) - p(-\frac{1}{2}, \uparrow)}{p_{3/2} + p(-\frac{3}{2}, \uparrow) + \frac{1}{2}p_{-1/2}} \tag{10}$$
$$V_{L1} = \frac{p(-\frac{3}{2}, \downarrow) - p(-\frac{1}{2}, \downarrow)}{2p_{3/2} + 2p(-\frac{3}{2}, \uparrow) + p(-\frac{1}{2}, \downarrow) + p(-\frac{3}{2}, \downarrow)} \tag{11}$$
$$p(-\frac{3}{2}, \uparrow) + p(-\frac{3}{2}, \downarrow) = p_{-3/2} \tag{12}$$
$$p(-\frac{1}{2}, \uparrow) + p(-\frac{1}{2}, \downarrow) = p_{-1/2} \tag{13}$$

Set of equations for $+\frac{1}{2}, +\frac{3}{2}$ subdomain:

$$V_n^{ms=+\frac{1}{2}} = \frac{p(\frac{1}{2}, \downarrow) - p(\frac{1}{2}, \uparrow)}{p_{-3/2} + p(\frac{3}{2}, \uparrow) + \frac{1}{2}p_{1/2}} \tag{14}$$
$$V_{R1} = \frac{p(\frac{3}{2}, \downarrow) - p(\frac{1}{2}, \downarrow)}{2p_{-3/2} + 2p(\frac{3}{2}, \uparrow) + p(\frac{1}{2}, \downarrow) + p(\frac{3}{2}, \downarrow)} \tag{15}$$
$$p(\frac{3}{2}, \uparrow) + p(\frac{3}{2}, \downarrow) = p_{3/2} \tag{16}$$
$$p(\frac{1}{2}, \uparrow) + p(\frac{1}{2}, \downarrow) = p_{1/2} \tag{17}$$

### 3. Solution $m_s = -\frac{1}{2}, -\frac{3}{2}$

$$
\begin{aligned}
p(-\frac{3}{2},\downarrow) &= \frac{4V_{L1}p_{3/2} + 0.5V_n\left(V_{L1}+1\right)\left(p_{-1/2}+2p_{3/2}\right) + p_{-1/2}\left(V_{L1}+1\right) + p_{-3/2}\left(4V_{L1}+V_n^-\left(V_{L1}+1\right)\right)}{2V_{L1}+V_n\left(V_{L1}+1\right)+2} \\
p(-\frac{1}{2},\downarrow) &= \frac{-2V_{L1}V_n^-p_{3/2} - V_n^-p_{-3/2}(V_{L1}-1) + 0.5V_n^-\left(V_{L1}+1\right)\left(p_{-1/2}+2p_{3/2}\right) + p_{-1/2}(V_{L1}+1)}{2V_{L1}+V_n^-\left(V_{L1}+1\right)+2} \\
(p-\frac{3}{2},\uparrow) &= -\frac{4V_{L1}p_{3/2} + 0.5V_n^-\left(V_{L1}+1\right)(p_{-1/2}+2p_{3/2}) + p_{-1/2}(V_{L1}+1) + 2p_{-3/2}(V_{L1}-1)}{2V_{L1}+V_n(V_{L1}+1)+2} \\
p(-\frac{1}{2},\uparrow) &= \frac{2V_{L1}V_n^-p_{3/2} + V_n^-p_{-3/2}(V_{L1}-1) - 0.5V_n^-\left(V_{L1}+1\right)(p_{-1/2}+2p_{3/2})}{2V_{L1}+V_n^-\left(V_{L1}+1\right)+2} + \\
&\quad + \frac{p_{-1/2}(V_{L1}+V_n^-\left(V_{L1}+1\right)+1)}{2V_{L1}+V_n^-\left(V_{L1}+1\right)+2}
\end{aligned}
\tag{18}
$$

Which could be further simplified:

$$
\begin{aligned}
p(-\frac{3}{2},\downarrow) &= \frac{(p_{-3/2}+p_{3/2})(4V_{L1}+V_n^-V_{L1}+V_n^-) + p_{-1/2}(0.5V_n^-+1)(V_{L1}+1)}{\left(V_n^-+2\right)\left(V_{L1}+1\right)} \\
p(-\frac{3}{2},\uparrow) &= -\frac{p_{3/2}(4V_{L1}+V_n^-+V_n^-V_{L1}) + 2p_{-3/2}(V_{L1}-1) + p_{-1/2}(0.5V_n^-+1)(V_{L1}+1)}{\left(V_n^-+2\right)\left(V_{L1}+1\right)} \\
p(-\frac{1}{2},\downarrow) &= \frac{\left(p_{-3/2}+p_{3/2}\right)V_n^-(1-V_{L1}) + p_{-1/2}(0.5V_n^-+1)(V_{L1}+1)}{\left(V_n^-+2\right)\left(V_{L1}+1\right)} \\
p(-\frac{1}{2},\uparrow) &= \frac{\left(p_{-3/2}+p_{3/2}\right)V_n^-\left(V_{L1}-1\right) + p_{-1/2}\left(0.5V_n^-+1\right)\left(V_{L1}+1\right)}{\left(V_n^-+2\right)\left(V_{L1}+1\right)}
\end{aligned}
\tag{19}
$$

### 4. Solution for $m_s = +\frac{1}{2}, +\frac{3}{2}$

The solution from the positive subdomain equations is symmetric ($3/2 \leftrightarrow -3/2$, $-1/2 \rightarrow 1/2$, $V_n^- \rightarrow V_n^+$, $V_L \rightarrow V_R$).

| Group | Atom | $T_2^*$ ($\mu$s) (-3/2; | -1/2; | +1/2; | +3/2) | DOP (A1) | DOP (A2) |
|---|---|---|---|---|---|---|---|
| II | 8 MHz Si | 34(2) | 22(1) | 46(1) | 230(35) | $94.6 \pm 4.0\,\%$ | $86.5 \pm 3.3\,\%$ |
| III | 4 MHz C | 55(8) | 31(5) | 134(26) | 347(46) | – | – |
| IV | 2 MHz Si | 75(3) | 125(10) | 397(19) | 498(42) | $98.7 \pm 6.0\,\%$ | $88.3 \pm 4.7\,\%$ |
| VI | 0.6 MHz Si | 868(102) | – | – | – | $47.1 \pm 6.0\,\%$ | $0.1 \pm 4.7\,\%$ |

TABLE I. Qubit performance at the GSLAC.

## III. MEASURING THE DEPHASING TIME

For determination of $T_2^*$ we used the following sequence. We start with 10 µs of 728 nm illumination (70 µW) to make sure the V2 is in its negative charge state. This is followed by initialization of the electron and nuclear spin as described in the main text, i.e. 100 µs of A1 (A2) resonant excitation (10 nW) and MW resonant to the $R$-transition to initialize into $|-3/2,\downarrow\rangle$ ($|-1/2,\downarrow\rangle$). For initialization into $m_s = +1/2$ and $m_s = +1/2$ we apply subsequent MW $\pi$-pulses to the higher electron levels.

After initialization of the system we apply a $\frac{\pi}{2} - \tau - \frac{\pi}{2}$ pulse sequence, slightly off-resonant with the nuclear spin transition in the corresponding electron sublevel. The usage of slightly de-tuned frequencies leads to an oscillating signal which can be fitted more precisely than a pure exponential decay. Furthermore, a $\pi$-phase can be added to the the second $\frac{\pi}{2}$-pulse, inverting the direction of rotation on the Bloch sphere. To project the nuclear spin state to a measureable electron state, a nuclear spin dependent MW $\pi$-pulse is used on the electron state (CNOT). Finally, the system is read out by the A2 laser, because this transition has a slightly higher cyclicity and is therefore brighter. By subtracting two subsequent measurements with opposite phase in the second $\frac{\pi}{2}$-pulse, common noise due to e.g. laser power fluctuations or drifts in the system, can be reduced.

We conducted those measurements on nuclear spins of group II, III, IV and IV. However, due to the weak polarization of the group VI nuclear spin in the $m_s = -1/2$-state it was not possible to measure the data in a decent quality. All data is shown in Fig. 1. Extracted values of $T_2^*$ can be found in Tab. I.

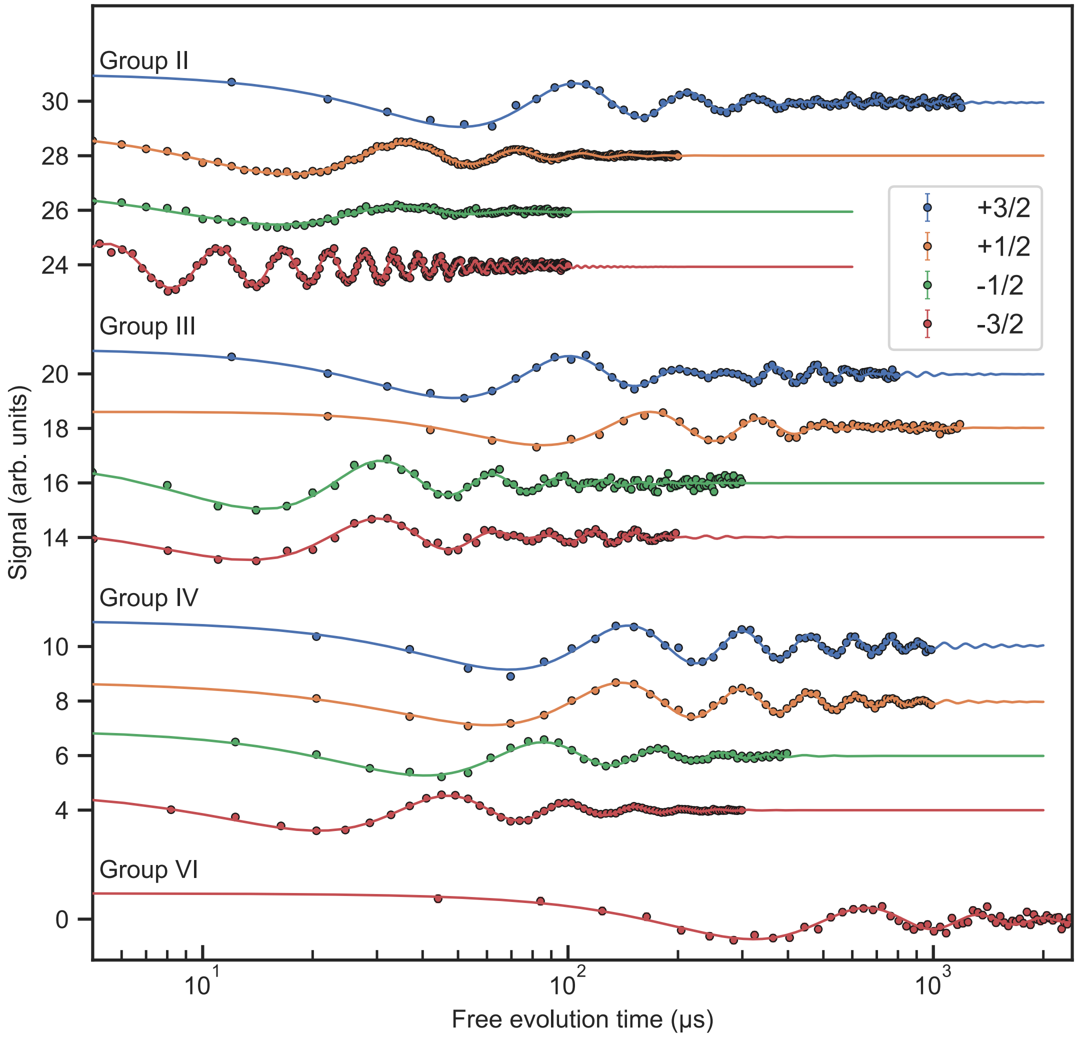


FIG. 1. Measured Ramsey decay on nuclear spins of group II, III, IV and VI. All data in normalized to an amplitude of 1. Colors indicate the electron spin state. All measurements are plotted with an offset of 2 to the next. Between groups an additional offset of 2 is added.

## IV. PERTURBATION ANALYSIS FOR V2 EPR AND NMR TRANSITIONS AROUND GSLAC

The full Hamiltonian $H$ of the V2 centre ground state in 4H-SiC crystal could be split by secular approximation into two parts:

$$H_{||} = DS_z^2 + \gamma_e BS_z + S_z A_{zz} I_z + S_z A_{zx} I_x + S_z A_{zy} I_y \tag{20}$$

and non secular part:

$$H_{\perp} = S_x A_{xx} I_x + S_y A_{yy} I_y + S_x A_{xz} I_z + S_y A_{yz} I_z \tag{21}$$

We use a secular approximation to find the zero order terms in the perturbation theory, and we focus now on four different spin subspaces: $m_s = -3/2, -1/2, 1/2, +3/2$.

The energy solutions are:

For $E_{m_s,\downarrow/\uparrow} = m_s^2 D - m_s \gamma B \pm \frac{1}{4}\sqrt{(\omega_L + m_s A_{zz})^2 + (m_s A_{zx})^2 + (m_s A_{zy})^2}$ for the perturbation analysis we take only the longitudinal part for zero order energies (for simplicity): $E_{m_s,\downarrow/\uparrow} = m_s^2 D - m_s \gamma B \pm \frac{1}{4}(\omega_L + m_s A_{zz})$, and we will include the secular $A_{zx} S_z I_x$ terms in the perturbation. The second order perturbations for the levels $m_s = -3/2$ and $m_s = +3/2$ only is perturbed by nuclear sublevels and by subleves with $m_s = -1/2$ and $m_s = +1/2$, (we neglect

$A_{xz}$ terms). First order perturbation are equal to zero (in case the eigenstates are perfectly aligned with Z axis), since $\langle n|I_{x/y}|n\rangle = 0$. The energy perturbations to the zero order solutions for $m_s = -3/2$ are:

$$\begin{aligned}
\Delta E^{(2)}_{-3/2,\uparrow} &= \underbrace{-\frac{(\frac{3}{4}A_{zx})^2}{\frac{3}{2}A_{zz}}}_{\text{hyperfine } S_zI_x} + \underbrace{0}_{S_xI_z \text{ microwave transitions}} - \underbrace{\frac{(\frac{\sqrt{3}}{4})^2(A_{xx}+A_{yy})^2}{\gamma_e B + A_{zz} - 2D}}_{S_xI_x \text{ and } S_yI_y \text{ construcitve}} \\
\Delta E^{(2)}_{-3/2,\downarrow} &= \underbrace{+\frac{(\frac{3}{4}A_{zx})^2}{\frac{3}{2}A_{zz}}}_{\text{hyperfine } S_zI_x} + \underbrace{0}_{S_xI_z \text{ microwave transitions}} - \underbrace{\frac{(\frac{\sqrt{3}}{4})^2(A_{xx}-A_{yy})^2}{\gamma_e B - A_{zz} - 2D}}_{S_xI_x \text{ and } S_yI_y \text{ destructive}}
\end{aligned} \tag{22}$$

For $m_s = +3/2$ similarly:

$$\begin{aligned}
\Delta E^{(2)}_{+3/2,\downarrow} &= \underbrace{-\frac{(\frac{3}{4}A_{zx})^2}{\frac{3}{2}A_{zz}}}_{\text{hyperfine } S_zI_x} + \underbrace{\frac{(\frac{\sqrt{3}}{4})^2(A_{xx}+A_{yy})^2}{\gamma_e B - A_{zz} + 2D}}_{S_xI_x \text{ and } S_yI_y \text{ constructive}} \\
\Delta E^{(2)}_{+3/2,\uparrow} &= \underbrace{+\frac{(\frac{3}{4}A_{zx})^2}{\frac{3}{2}A_{zz}}}_{\text{hyperfine } S_zI_x} + \underbrace{\frac{(\frac{\sqrt{3}}{4})^2(A_{xx}-A_{yy})^2}{\gamma_e B + A_{zz} + 2D}}_{S_xI_x \text{ and } S_yI_y \text{ destructive}}
\end{aligned} \tag{23}$$

For the levels $m_s = \pm 1/2$ we need to consider more terms, since they interact both with 1/2 and 3/2 subdomains, as well as within their nuclear subdomains, but as already understood, we neglect terms with $A_{xz}S_xI_z$ and only keep the non zero terms,

The energy perturbations to the zero order solutions for $m_s = -1/2$ are:

$$\begin{aligned}
\Delta E^{(2)}_{-1/2,\uparrow} &= \underbrace{-\frac{(\frac{1}{4}A_{zx})^2}{\frac{1}{2}A_{zz}}}_{\text{hyperfine } S_zI_x} - \underbrace{\frac{(\frac{1}{2})^2(A_{xx}+A_{yy})^2}{\gamma_e B}}_{S_xI_x \text{ and } S_yI_y \text{ constr. with } m_s=+1/2,\downarrow} + \underbrace{\frac{(\frac{\sqrt{3}}{4})^2(A_{xx}-A_{yy})^2}{\gamma_e B - A_{zz} - 2D}}_{S_xI_x \text{ and } S_yI_y \text{ destr. with } m_s=-3/2,\downarrow} \\
\Delta E^{(2)}_{-1/2,\downarrow} &= \underbrace{+\frac{(\frac{1}{4}A_{zx})^2}{\frac{1}{2}A_{zz}}}_{\text{hyperfine } S_zI_x} - \underbrace{\frac{(\frac{1}{2})^2(A_{xx}-A_{yy})^2}{\gamma_e B}}_{S_xI_x \text{ and } S_yI_y \text{ destr. with } m_s=+1/2,\uparrow} + \underbrace{\frac{(\frac{\sqrt{3}}{4})^2(A_{xx}+A_{yy})^2}{\gamma_e B + A_{zz} - 2D}}_{S_xI_x \text{ and } S_yI_y \text{ constr. with } m_s=-3/2,\uparrow}
\end{aligned} \tag{24}$$

For $m_s = +1/2$ :

$$\begin{aligned}
\Delta E^{(2)}_{+1/2,\downarrow} &= -\underbrace{\frac{(\frac{1}{4}A_{zx})^2}{\frac{1}{2}A_{zz}}}_{\text{hyperfine } S_zI_x} + \underbrace{\frac{(\frac{1}{2})^2(A_{xx}+A_{yy})^2}{\gamma_e B}}_{S_xI_x \text{ and } S_yI_y \text{ constr. with } m_s=-1/2,\uparrow} - \underbrace{\frac{(\frac{\sqrt{3}}{4})^2(A_{xx}-A_{yy})^2}{\gamma_e B + A_{zz} + 2D}}_{S_xI_x \text{ and } S_yI_y \text{ destr. with } m_s=+3/2,\uparrow} \\
\Delta E^{(2)}_{+1/2,\uparrow} &= \underbrace{+\frac{(\frac{1}{4}A_{zx})^2}{\frac{1}{2}A_{zz}}}_{\text{hyperfine } S_zI_x} - \underbrace{\frac{(\frac{1}{2})^2(A_{xx}-A_{yy})^2}{\gamma_e B}}_{S_xI_x \text{ and } S_yI_y \text{ destr. with } m_s=-1/2,\downarrow} - \underbrace{\frac{(\frac{\sqrt{3}}{4})^2(A_{xx}+A_{yy})^2}{\gamma_e B - A_{zz} + 2D}}_{S_xI_x \text{ and } S_yI_y \text{ constr. with } m_s=+3/2,\downarrow}
\end{aligned} \tag{25}$$

This is expressed in the figure 2.

As one can see the endor frequencies could be simplifed in the case $A_{xx} \approx A_{yy}$ as

$$\begin{aligned}
\nu_{-3/2} &\approx \frac{3}{2}A_{zz} + \frac{3A_{zx}^2}{4A_{zz}} + \frac{3}{16}\frac{(A_{xx}+A_{yy})^2}{(\gamma_e B + A_{zz} - 2D)} \\
\nu_{+3/2} &\approx \frac{3}{2}A_{zz} + \frac{3A_{zx}^2}{4A_{zz}} - \frac{3}{16}\frac{(A_{xx}+A_{yy})^2}{(\gamma_e B - A_{zz} + 2D)} \\
\nu_{-1/2} &\approx \frac{1}{2}A_{zz} + \frac{A_{zx}^2}{4A_{zz}} + \frac{3}{16}\frac{(A_{xx}+A_{yy})^2}{(\gamma_e B + A_{zz} - 2D)} + \frac{1}{4}\frac{(A_{xx}+A_{yy})^2}{\gamma_e B} \\
\nu_{+1/2} &\approx \frac{1}{2}A_{zz} + \frac{A_{zx}^2}{4A_{zz}} - \frac{3}{16}\frac{(A_{xx}+A_{yy})^2}{(\gamma_e B - A_{zz} + 2D)} - \frac{1}{4}\frac{(A_{xx}+A_{yy})^2}{\gamma_e B}
\end{aligned} \tag{26}$$

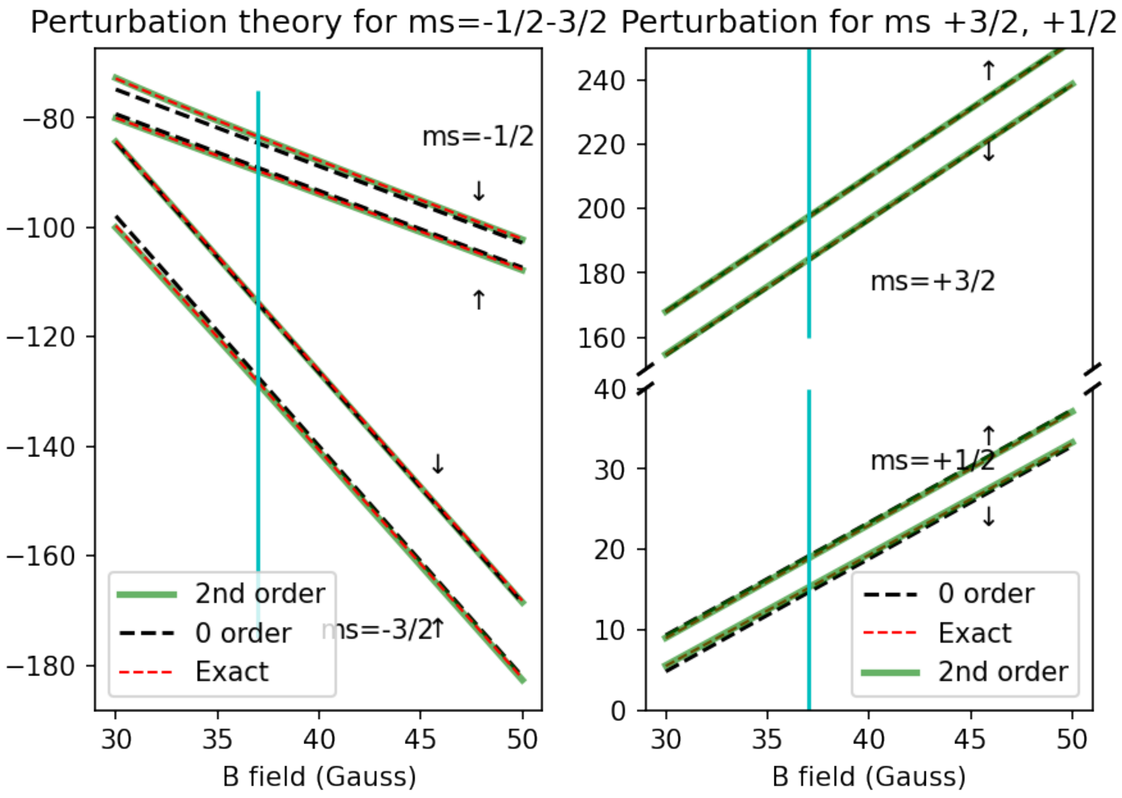


FIG. 2. Perturbation of the energy levels for SiC $S = 3/2$, and $I = 1/2$. $A_{zz} = 9$ MHz, $A_{xx} = A_{yy} = 8$ MHz, $A_{zx} = 1$

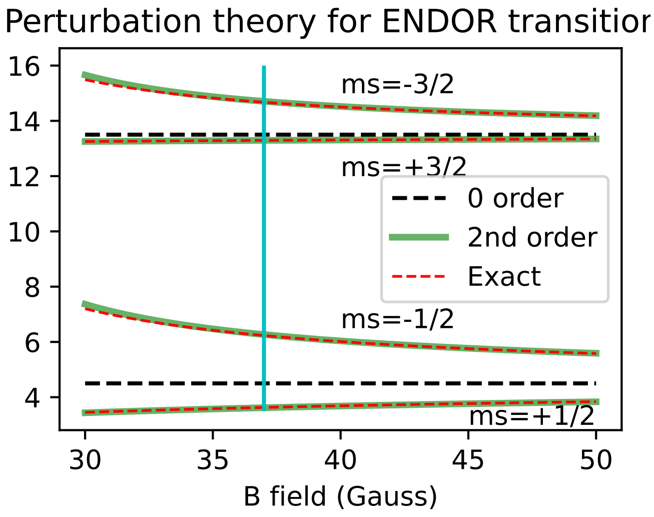


FIG. 3. Perturbation of the ENDOR transition frequencies for SiC $S = 3/2$, and $I = 1/2$. $A_{zz} = 9$ MHz, $A_{xx} = A_{yy} = 8$ MHz, $A_{zx} = 1$

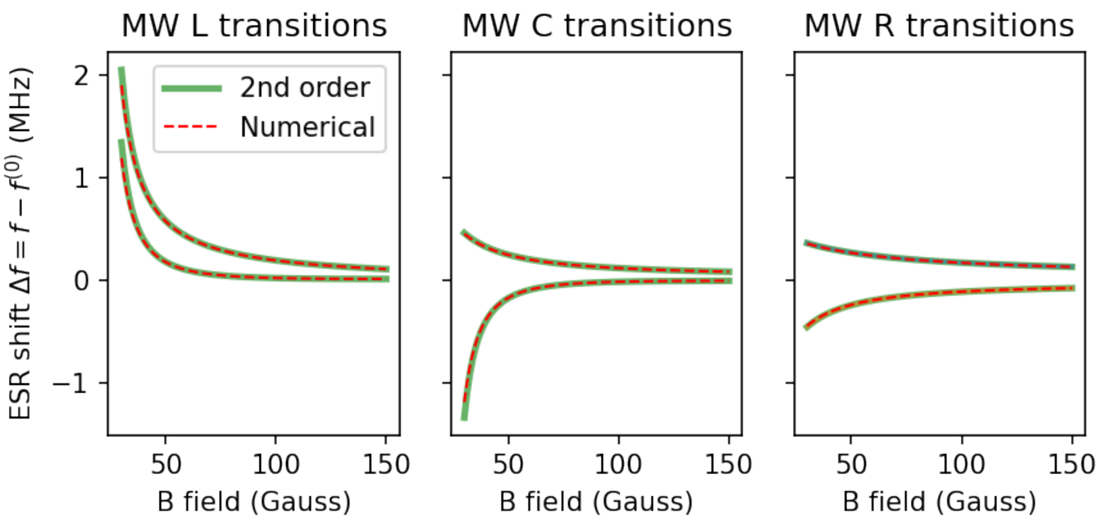


FIG. 4. Perturbation of the ESR transition frequencies for SiC $S = 3/2$, and $I = 1/2$. $A_{zz} = 9$ MHz, $A_{xx} = A_{yy} = 8$ MHz, $A_{zx} = 1$

This is expressed in the figure 3.

The ESR transitions then are perturbed as well, by the value:

$$\begin{aligned}
f_{L1} &\approx E^{(2)}_{-1/2,\downarrow} - E^{(2)}_{-3/2,\downarrow} = \gamma_e B - 2D - \frac{1}{2}A_{zz} - \frac{A_{zx}^2}{4A_{zz}} + \frac{3}{16}\cdot\frac{(A_{xx}+A_{yy})^2}{\gamma_e B - 2D + A_{zz}} \\
f_{L2} &\approx E^{(2)}_{-1/2,\uparrow} - E^{(2)}_{-3/2,\uparrow} = \gamma_e B - 2D + \frac{1}{2}A_{zz} + \frac{A_{zx}^2}{4A_{zz}} + \frac{3}{16}\cdot\frac{(A_{xx}+A_{yy})^2}{\gamma B - 2D + A_{zz}} - \frac{(A_{xx}+A_{yy})^2}{4\gamma_e B} \\
f_{C1} &\approx E^{(2)}_{1/2,\uparrow} - E^{(2)}_{-1/2,\uparrow} = \gamma_e B + \frac{1}{2}A_{zz} + \frac{A_{zx}^2}{4A_{zz}} - \frac{3}{16}\cdot\frac{(A_{xx}+A_{yy})^2}{\gamma_e B - A_{zz} + 2D} + \frac{(A_{xx}^2+A_{yy}^2)^2}{4\gamma_e B} \\
f_{C2} &\approx E^{(2)}_{1/2,\downarrow} - E^{(2)}_{-1/2,\downarrow} = \gamma_e B - \frac{1}{2}A_{zz} - \frac{A_{zx}^2}{4A_{zz}} - \frac{3}{16}\cdot\frac{(A_{xx}+A_{yy})^2}{\gamma_e B + A_{zz} - 2D} + \frac{(A_{xx}^2+A_{yy}^2)^2}{4\gamma_e B} \\
f_{R1} &\approx E_{3/2\uparrow} - E_{1/2\uparrow} = 2D + \gamma_e B + \frac{1}{2}A_{zz} + \frac{A_{zx}^2}{4A_{zz}} + \frac{3}{16}\cdot\frac{(A_{xx}+A_{yy})^2}{\gamma_e B - A_{zz} + 2D} \\
f_{R2} &\approx E_{3/2\downarrow} - E_{1/2\downarrow} = 2D + \gamma_e B - \frac{1}{2}A_{zz} - \frac{A_{zx}^2}{4A_{zz}} + \frac{3}{16}\cdot\frac{(A_{xx}+A_{yy})^2}{\gamma_e B - A_{zz} + 2D} - \frac{(A_{xx}+A_{yy})^2}{4\gamma_e B}
\end{aligned} \tag{27}$$

This is expressed in the figure 4 which shows a nice agreement between the transition frequencies numerically calculated and perturbation theory. In conclusion we find that the deviations in the case of 8 Mhz spin are on the order of 1MHz, while the precision in our measurements is below 10-100 kHz, depending on the averaging time.

## V. HYPERFINE ENHANCEMENT

To better understand the systems dynamic close to the ground-state level-anticrossing, we outline the calculations to obtain an analytical expression of the hyperfine enhancement. Similar calculations were first published in [2, 3] for the NV$^-$-system in diamond. Here we sketch out the calculations for the present spin-3/2 system.

The system Hamiltonian consists of the zero-field splitting (ZFS), electron Zeeman effect (EZ), nuclear Zeeman effect (NZ) and hyperfine interaction (HFI)

$$H = H_{\|} + H_{\perp} \tag{28}$$

$$H_{\|} = \underbrace{\Delta S_z^2}_{\text{ZFS}} + \underbrace{\gamma_e B_z S_z}_{\text{EZ}} + \underbrace{\gamma_n B_z I_z}_{\text{NZ}} + \underbrace{A_{\|} S_z I_z}_{\text{HFI}} \tag{29}$$

$$H_{\perp} = \underbrace{A_{xx} S_x I_x + A_{yy} S_y I_y}_{\text{spin-flipping HFI}} \tag{30}$$

which can be expressed in matrix form as:

$$H = \begin{pmatrix} D & 0 & 0 & DQ & 0 & 0 & 0 & 0 \\ 0 & D & ZQ & 0 & 0 & 0 & 0 & 0 \\ 0 & ZQ & D & 0 & 0 & DQ & 0 & 0 \\ DQ & 0 & 0 & D & ZQ & 0 & 0 & 0 \\ 0 & 0 & 0 & ZQ & D & 0 & 0 & DQ \\ 0 & 0 & DQ & 0 & 0 & D & ZQ & 0 \\ 0 & 0 & 0 & 0 & 0 & ZQ & D & 0 \\ 0 & 0 & 0 & 0 & DQ & 0 & 0 & D \end{pmatrix}$$

Here, three different kind of entries occur. Entries on the diagonal ($D$), entries which correspond to a spin flip-flop ($ZQ \propto A_{xx} + A_{yy}$, standing for zero-quantum) and entries corresponding to double-quantum transitions ($DQ \propto A_{xx} - A_{yy}$). Note that $DQ = 0$ when $A_{xx} - A_{yy} = 0$. Then the Hamiltonian can be diagonalized by rotating the three ZQ-subspaces indicated by blue color. This requires the unitary transformation

$$U_{ZQ} = \exp\left(-i(\sigma_y^l \vartheta^l + \sigma_y^c \vartheta^c + \sigma_y^r \vartheta^r)\right) \tag{31}$$

where we defined

$$\sigma_y^l = i\left(\left|-\frac{1}{2},-\frac{1}{2}\right\rangle\left\langle-\frac{3}{2},\frac{1}{2}\right| - \left|-\frac{3}{2},\frac{1}{2}\right\rangle\left\langle-\frac{1}{2},-\frac{1}{2}\right|\right), \tag{32}$$

$$\sigma_y^c = i\left(\left|\frac{1}{2},-\frac{1}{2}\right\rangle\left\langle-\frac{1}{2},\frac{1}{2}\right| - \left|-\frac{1}{2},\frac{1}{2}\right\rangle\left\langle\frac{1}{2},-\frac{1}{2}\right|\right), \tag{33}$$

$$\sigma_y^r = i\left(\left|\frac{3}{2},-\frac{1}{2}\right\rangle\left\langle\frac{1}{2},\frac{1}{2}\right| - \left|\frac{1}{2},\frac{1}{2}\right\rangle\left\langle\frac{3}{2},-\frac{1}{2}\right|\right). \tag{34}$$

To obtain the rotation angles, we rotate the Hamiltonian and set the ZQ entries to 0

$$H' = U_{ZQ} H U_{ZQ}^{\dagger} \tag{35}$$

$$\tan(2\vartheta^l) = -\frac{\frac{\sqrt{3}}{2}(A_{xx} + A_{yy})}{-A + B_z(\gamma_e - \gamma_n) + 2\Delta} \tag{36}$$

$$\tan(2\vartheta^c) = -\frac{A_{xx} + A_{yy}}{B_z(\gamma_e - \gamma_n)} \tag{37}$$

$$\tan(2\vartheta^r) = -\frac{\frac{\sqrt{3}}{2}(A_{xx} + A_{yy})}{A + B_z(\gamma_e - \gamma_n) - 2\Delta} \tag{38}$$

$$\tag{39}$$

We now apply the transformation $U_{ZQ}(\vartheta^l, \vartheta^c, \vartheta^r)$ to the Interaction Hamiltonian in the rotating frame $H_{RF} = B_{RF}(\gamma_e S_x + \gamma_n I_x)$ and extract the entries which correspond to nuclear spin transitions. These transitions are enhanced

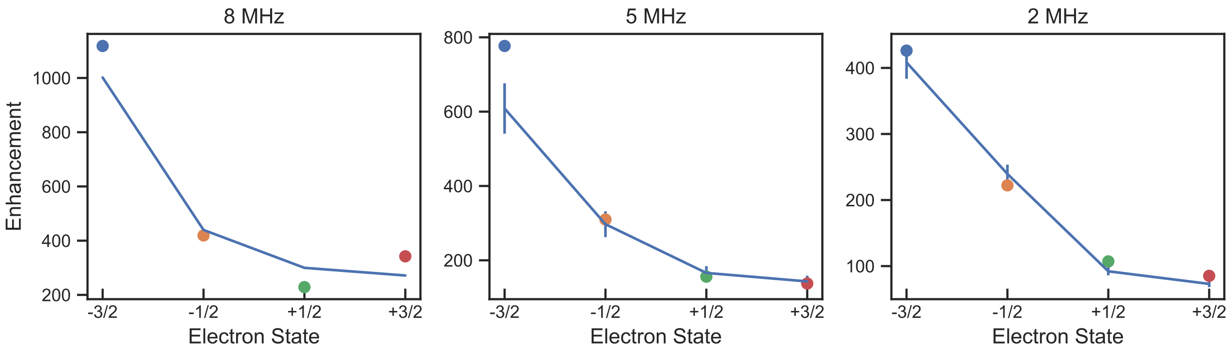


FIG. 5. Comparison of theoretically predicted and experimentally measured nuclear rabi frequencies for nuclear spins of various coupling strength.

by a different factor for each electron-subspace:

$$\alpha_{+\frac{3}{2}} = \sqrt{3}\frac{\gamma_e}{\gamma_n}\sin(\vartheta^r) + \cos(\vartheta^r) \tag{40}$$

$$\alpha_{+\frac{1}{2}} = \frac{\gamma_e}{\gamma_n}\left(+2\sin(\vartheta^c)\cos(\vartheta^r) - \sqrt{3}\sin(\vartheta^c)\cos(\vartheta^r)\right) + \cos(\vartheta^c)\cos(\vartheta^r) \tag{41}$$

$$\alpha_{-\frac{1}{2}} = \frac{\gamma_e}{\gamma_n}\left(-2\sin(\vartheta^c)\cos(\vartheta^l) + \sqrt{3}\sin(\vartheta^l)\cos(\vartheta^c)\right) + \cos(\vartheta^l)\cos(\vartheta^c) \tag{42}$$

$$\alpha_{-\frac{3}{2}} = -\sqrt{3}\frac{\gamma_e}{\gamma_n}\sin(\vartheta^l) + \cos(\vartheta^l) \tag{43}$$

The gyromagnetic enhancement can be extracted from Rabi oscialltions of electron and nuclear spins, where the Rabi frequency is propotional to the strength of the drive field $B_1$.

$$\Omega_L \propto \gamma_e B_1 \frac{\sqrt{3}}{2}\begin{pmatrix} 0 & 1 \\ 1 & 0 \end{pmatrix} \tag{44}$$

$$\Omega_n \propto \alpha\gamma_n B_1 \frac{1}{2}\begin{pmatrix} 0 & 1 \\ 1 & 0 \end{pmatrix}, \tag{45}$$

where $\Omega_L$ is the experimentally observed Rabi frequency of the left electron transition, $\Omega_n$ is the nuclear rabi frequency and $\alpha$ is the enhancement of the gyromagnetic ratio. Assuming, that $B_1$ is the same at both transition frequencies, this can be rearranged to

$$\frac{2\Omega_L}{\sqrt{3}\gamma_e} = \frac{2\Omega_n}{\alpha\gamma_n}. \tag{46}$$

which directly leads to the enhancement factor

$$\alpha = \sqrt{3}\frac{\Omega_n}{\Omega_L}\frac{\gamma_e}{\gamma_n}. \tag{47}$$

Fig. 5 compares the analytical results of $\alpha$ (eq. 40 - 43) with the experimentally obtained enhancement (eq. 47) of various nuclear spins.

## VI. EXPERIMENTAL SETUP

All experiments were performed at cryogenic temperature <10 K in a Montana Instruments cryostation. A home build confocal microscope was used to optically excite single V2 centers and detect the red-shifted phonon side band. Off-resonant excitation was performed with a 728nm diode laser (Toptica iBeam Smart). For resonant excitation we used an external cavity tunable diode laser (Toptica DL Pro), which was split and frequency shifted by two AOMs to address both optical transitions. Laser photons are filtered by two tunable long-pass filters (Semrock TLP01-995). The used photon detectors are fiber coupled superconducting nanowire single-photon detectors (SNSPDs) from Photon Spot. The measurements were controlled via qudi, a modular python suite for control of laboratory experiments [4].

For most of our measurements, we used 10 nW excitation power before the cryostation. From the simulations we extract that the amplitude of the magnetic field of the microwave is up to 2 mT at the defect location, with usual amplitudes around 0.4 mT

## VII. SILICON CARBIDE SAMPLE

Ultra-high purity homoepitaxial layers of 4H-SiC were grown on a-plane substrates in a hot-wall chemical vapor deposition (CVD) reactor, employing gas foil rotation of the substrate. The growth process utilized chloride-based chemistry, employing trichlorosilane and propane with a natural isotopic abundance of silicon and carbon. The maximum thickness of the layers reached 10 µm, with n-type nitrogen doping concentration of 7-9 $\times 10^{13}\,\mathrm{cm}^{-3}$. The thickness and doping concentration of the epitaxial layers were assessed through Fourier-transformed infrared reflectivity (FTIR) and capacitance-voltage (CV) measurements, respectively. The surface of the layers exhibited exceptional smoothness, devoid of any discernible morphological defects. Silicon vacancies were generated by electron irradiation at 2MeV with a fluence of 20kGy. After defect creation the sample was annealed at 600°C in Argon atmosphere for 30 min (heating: 5°C/min, cooling: -2.5°C/min).

Eventually, 8 solid immersion lenses (SILs) with diameter of 11 µm are milled into the substrate via a gallium focus-ion-beam. The recipe described in [5] was used. However, instead of the 50 nm Au-layer, a 10 nm Cr + 100 nm Au coating was used. We obtained about 20 randomly distributed V2 centers per SIL. The achieved optical linewidth of A1 and A2 transitions are about 100-150 MHz with a saturation countrate of 10-20 kHz in the phonon side band under resonant excitation.

## VIII. COMPARISON OF DFT CALCULATION WITH MEASURED DATA

We use the VASP software package to obtain an accurate spin density of the V2 center in a 1536-atom supercell model using 500 eV plane wave basis set, projector augmented-wave methods[6], and HSE06 functional[7]. The structural model is relaxed until the largest force is smaller than $10^{-3}$ e/Å. The finite-effect free hyperfine tensors are according to the method developed in Ref. [8]. In order to compare the results from the DFT calculation to the measurements, we plug in our hamiltonian model the calculated DFT couplings and extract from there the expected transition frequencies and compare them to the measured transitions. This way, we can identify the 6 most probable coupled nuclear spins for the studied defect.

## IX. UNCERTAINITY ON THE HYPERFINE TENSOR ELEMENTS FIT

In order to characterize the error on the fit, we fit the transtions 1000 times with random variations on the transition in the order of the incertainity on the peak position fit in the ODMR. Additionally, the initial guess of the fit is genarated randomly. Whith this statistics pool, we first-post select the fit parameters based on the fit fidelity (ie.norm of the transition frequency error vector). In the statistics, we can clearly see the different local minima as they represent steps in the achieved fidelity. Inside these local minima, we sometimes can identify other minima expressed by steps in the final values of the fit parameters. for each one tof these steps we then calculate the mean value and the standard deviation which we consider to be the fit error. The mean calculated value mean value is then used as initial guess for a final fit which gives us the final tensor values.


[1] R. Nagy, M. Niethammer, M. Widmann, Y.-C. Chen, P. Udvarhelyi, C. Bonato, J. U. Hassan, R. Karhu, I. G. Ivanov, N. T. Son, *et al.*, High-fidelity spin and optical control of single silicon-vacancy centres in silicon carbide, Nature communications **10**, 1 (2019).

[2] M. Chen, M. Hirose, and P. Cappellaro, Measurement of transverse hyperfine interaction by forbidden transitions, Phys. Rev. B **92**, 020101 (2015).

[3] S. Sangtawesin, C. McLellan, B. Myers, A. B. Jayich, D. Awschalom, and J. R. Petta, Hyperfine-enhanced gyromagnetic ratio of a nuclear spin in diamond, New Journal of Physics **18**, 083016 (2016).

[4] J. M. Binder, A. Stark, N. Tomek, J. Scheuer, F. Frank, K. D. Jahnke, C. Müller, S. Schmitt, M. H. Metsch, T. Unden, T. Gehring, A. Huck, U. L. Andersen, L. J. Rogers, and F. Jelezko, Qudi: A modular python suite for experiment control and data processing, SoftwareX **6**, 85 (2017).

[5] M. Widmann, S.-Y. Lee, T. Rendler, N. T. Son, H. Fedder, S. Paik, L.-P. Yang, N. Zhao, S. Yang, I. Booker, A. Denisenko, M. Jamali, S. A. Momenzadeh, I. Gerhardt, T. Ohshima, A. Gali, E. Janzén, and J. Wrachtrup, Coherent control of single spins in silicon carbide at room temperature, Nature Materials **14**, 164 (2015).

[6] P. E. Blöchl, Projector augmented-wave method, Phys. Rev. B **50**, 17953 (1994).

[7] J. Heyd, G. E. Scuseria, and M. Ernzerhof, Hybrid functionals based on a screened coulomb potential, **118**, 8207 (2003).

[8] I. Takács and V. Ivády, Accurate Hyperfine Tensors for Solid State Quantum Applications: Case of the NV Center in Diamond (2023), arXiv:2309.03983.
